# Supplementary material for: A platform for high performance photon correlation measurements
Source: arXiv:2003.09916 source file (2020-03-22)
Supplement: Supplementary file 1 [file SI.pdf]

Supporting information for

# A platform for high performance photon correlation measurements

Iman Esmaeil Zadeh*, Johannes W. N. Los, Ronan B. M. Gourgues, Jin Chang, Ali W. Elshaari, Julien Zichi, Yuri J. van Staaden, Jeroen Swens, Nima Kalhor, Antonio Guardiani, Yun Meng, Kai Zou, Sergiy Dobrovolskiy, Andreas W. Fognini, Dennis R. Schaart, Dan Dalacu, Philip J. Poole, Michael E. Reimer, Xiaolong Hu, Silvania F. Pereira, Val Zwiller, Sander N. Dorenbos

* i.esmaeilzadeh@tudelft.nl

## S1- High performance devices

### S1.1. Examples of high performance devices at various wavelength

Beside the detectors that are discussed in the main text, we measured other high performance devices at different wavelengths. Fig. S 1 shows examples of such detectors:

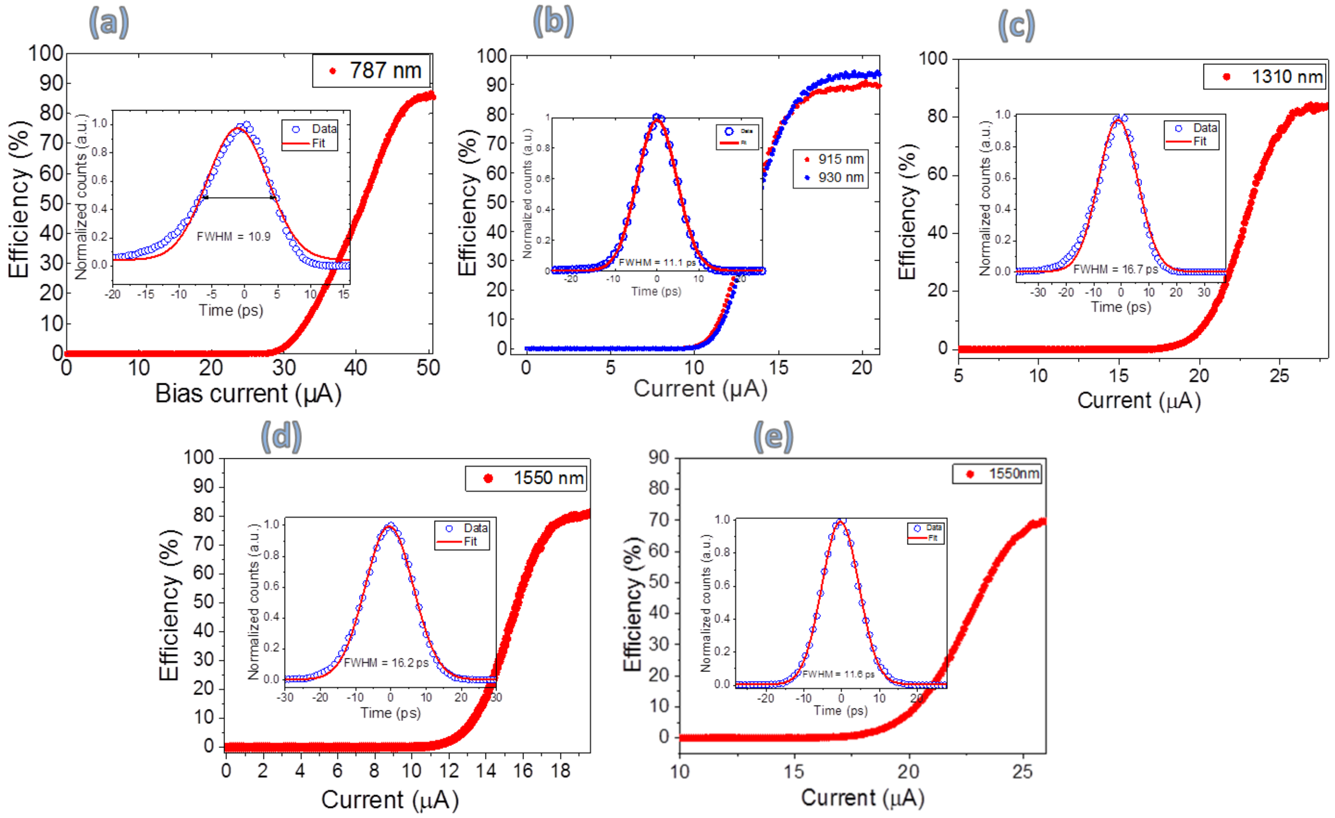


**Fig. S 1 Examples of efficient single-photon detectors at various wavelength and their corresponding time resolution.**

The detector that was measured at 787 nm (Fig. S 1(a)) had a nanowire linewidth of 100nm (designed), while other detectors (Fig. S 1 (b-e)) had nanowire widths of 70nm (designed) but different film thickness and compositions as discussed in the main text.

### S1.2. Performance comparison of small and big detectors

We fabricated small (diameter of 9 and 10 μm) and large detectors (diameter 20 μm) from a 11nm NbTiN film sputtered on a 4-inch wafer. The detectors were grouped together and their performance was evaluated. For the large detectors, apart from isolating broken devices (by a simple visual inspection), we selected the detectors at random.
Shown below, Fig. S 2, is the performance summary of 8 small dimeter detectors (measurements at λ = 878nm) and 8 randomly chosen large detectors (measured at λ = 937nm since the 878nm laser was damaged). The performance of the detectors are comparable: a high efficiency (~85%) and high critical current (35-45 μA). The small difference in critical currents (higher for larger detectors) can be attributed to thickness gradient along the 4-inch wafer and possible nanowire width variation due to fabrication parameters such as different proximity effects for large and small detectors.

(a)

| Detector# | Ic (μA) | Efficiency (%) | Design (widths-period- diameter) |
|---|---|---|---|
| S1 | 38.4 | 85 | w70p140-10μm |
| S2 | 39.2 | 88 | w70p140-9μm |
| S3 | 38.4 | 81 | w70p140-10μm |
| S4 | 39.5 | 90 | w70p140-10μm |
| S5 | 38.0 | 76 | w70p140-10μm |
| S6 | 36.6 | 85 | w70p140-9μm |
| S7 | 36 | 85 | w70p140-9μm |
| S8 | 39.5 | 82 | w70p140-9μm |

(b)

| Detector# | Ic(μA) | Efficiency (%) | Design (widths-period- diameter) |
|---|---|---|---|
| B1 | 44.5 | 87 | w70p140-20μm |
| B2 | 40.9 | 80 | w70p140-20μm |
| B3 | 44.2 | 87 | w70p140-20μm |
| B4 | 43.8 | 90 | w70p140-20μm |
| B5 | 39.1 | 76 | w70p140-20μm |
| B6 | 38.2 | 85 | w70p140-20μm |
| B7 | 44.5 | 85 | w70p140-20μm |
| B8 | 45 | 82 | w70p140-20μm |

**Fig. S 2, Critical current and efficiency of (a) 8 small detectors (9 and 10 micrometers in diameter) and (b) 8 randomly chosen large detectors with a diameter of 20μm (length of ~4.5 mm).**

# S2- Jitter

## S2.1. Jitter at high count-rate

The count rate of the detector can influence its jitter. We observed that rather than only detector count rate, the ratio of the detector count rate to the laser rep-rate influences the shape of the distribution. We attenuated pulses from a 50MHz pulsed laser to get different detection rates and carried out photon correlations at each point, the results of such measurements for a detector with the parallel high-pass filter, as shown in Fig. S 3(a), are presented in Fig. S 3(b). It can be observed that at low count-rates (below 0.1 × laser repetition-rate), SNSPD time jitter exhibit a typical single Gaussian distribution. However, as the count-rate increases, other peaks appear in the distribution. The observation of these peaks can be explained by the fact that when the recovery time of the bias current of SNSPD is longer than $\frac{1}{laser\ rep-rate}$ , subsequent detection events take place with an under-biased detector, while detection events which are temporally further away would experience detection with full bias current. The probability of detecting subsequent pulses (and hence the amplitude of their corresponding peak in the photon correlation distribution) depends on count-rate, being initially small and increasing as the count-rate increases. At the count rate gets close to the laser rep-rate, again the jitter starts to reduce as there is eventually only one possibility: all detection events are from subsequent pulses. By increasing the photon flux further, the latter case give us a distribution similar to the one shown in Figure 3d with 3.5 ps time jitter (main text).

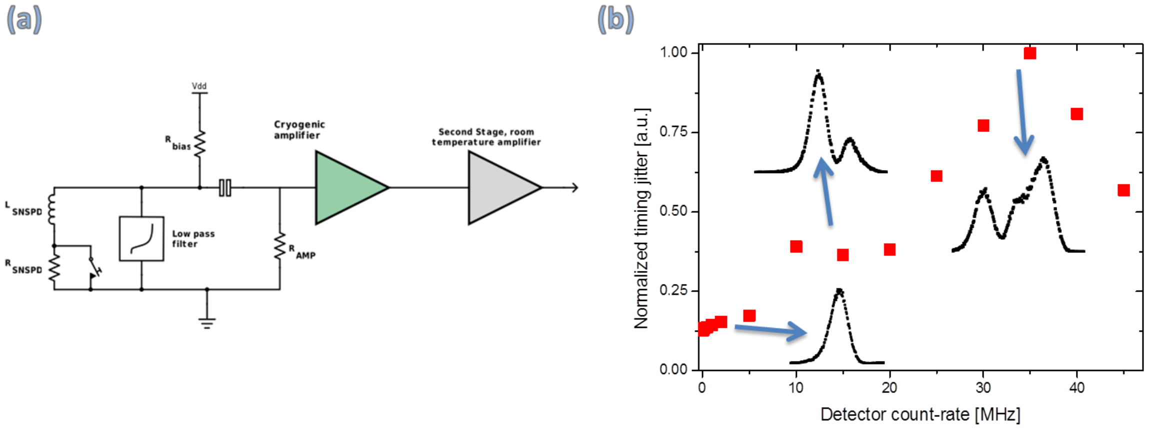


Fig. S 3, (a) A circuit schematic for the SNSPD with parallel high-pass filter (as discussed in the main text), (b) time jitter measurement versus countrate. For details see the text.

## S2.2. Contribution of laser optical pulses and the electronics on system time jitter

We have discussed about the correlation electronics used in our experiments elsewhere [1]. The electronics has a time jitter of ~2.5ps . However, the largest contribition to the system jitter (apart from detector itself) stems from the length of the optical pulses.To measure the contribution from the laser, we use a pulse autocorrelation setup as describe below: PulseCheck Autocorrelator was used to measure the pulse width of the Fianium WhiteLase Micro supercontinuum laser. PulseCheck Autocorrelator makes use of second-harmonic generation (SHG) to retrieve the pulse width by overlapping the laser pulse in a SHG crystal and generate a new pulse with twice the frequency of the input pulse. An interferometry scheme introduces a delay between the pulses previously split by a beam splitter and the SHG pulse energy versus delay is measured by a photomultiplier tube, as shown in Fig. S 4.

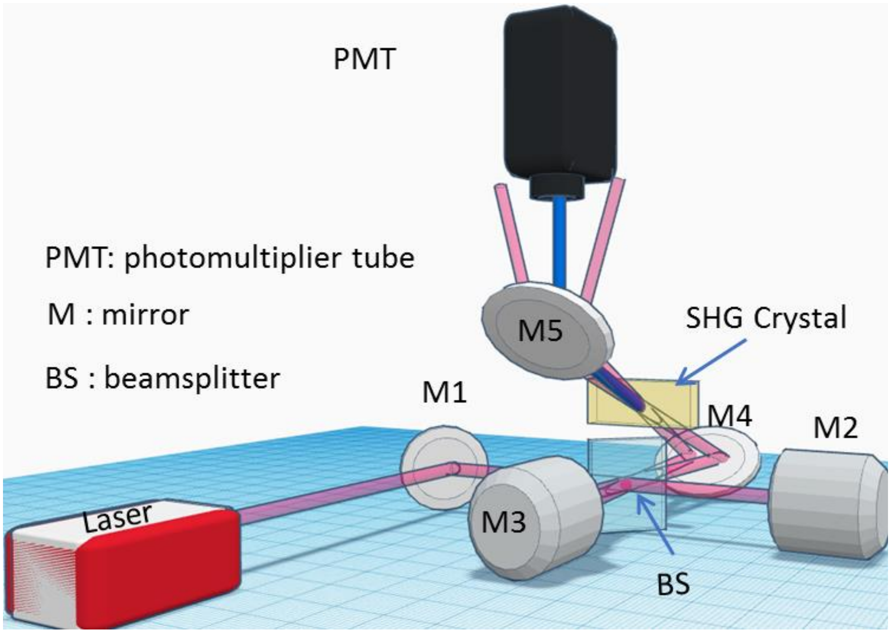


**Fig. S 4,** Sketch of PulseCheck Autocorrelator operated in non-collinear mode

From the Autocorrelation trace, Gaussian fitting is then performed and a Gaussian pulse width of 5.080ps is retrieved, see Fig. S 5. PulseCheck Autocorrelator was operated in non collinear mode in order to generate noise free SHG signal at the detector.

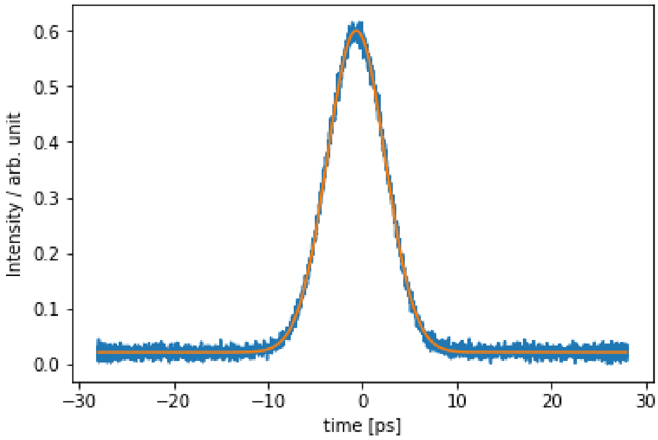


**Fig. S 5, Intensity Autocorrelation of Fianium WhiteLase Micro supercontinuum laser measurement (blue) and fit (orange) yielding a 5.080ps optical pulse length.**

## S2.3. Jitter versus trigger level

We measured time jitter as a function of trigger level for a detector with a minimum jitter of ~15.5ps (detector was ~500 µm in length). The results indicate that, when the noise level is lower or the pulse has steeper slope, the time jitter is improved. The time jitter remains within 15.5-22.5ps for trigger levels in the range of 10-80%. At much lower or higher trigger levels, the jitter would suffer from low signal to noise ratio.

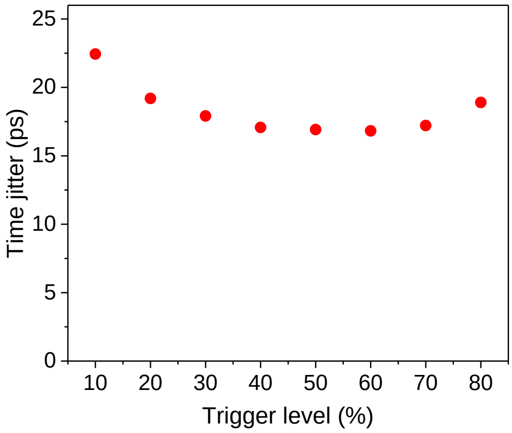


**Fig. S 6, time jitter vs trigger level for detector with a minimum jitter of ~15.5 ps.**

## S2.4. Jitter of two sectioned SNSPD

As described in the main text we fabricated two section detectors to study the influence of fabrication imperfections on the time jitter of SNSPDs. Below, in Fig. S 7(a) more SEM images of such an SNSPD with 70nm wide and 77nm wide sections are shown. We also fabricated detectors with 68nm wide and 70nm wide sections (only 2nm difference). Interestingly we can still observe the two peaks which we saw for the former case but in this case since the peaks are much narrower, to get a good fit, one cannot neglect the shoulder on the left side of the distribution which is possibly originated from detection in the nanowire bends, as reported in [2]. Shown in Fig. S 7 (b) is the photon correlation measurements for the two section detector with 68nm wide and 70nm wide sections at 3 different bias currents. Particularly at higher currents, where the two main peaks are narrow, the addition of third peak (as described above) is necessary to achieve a good fit.

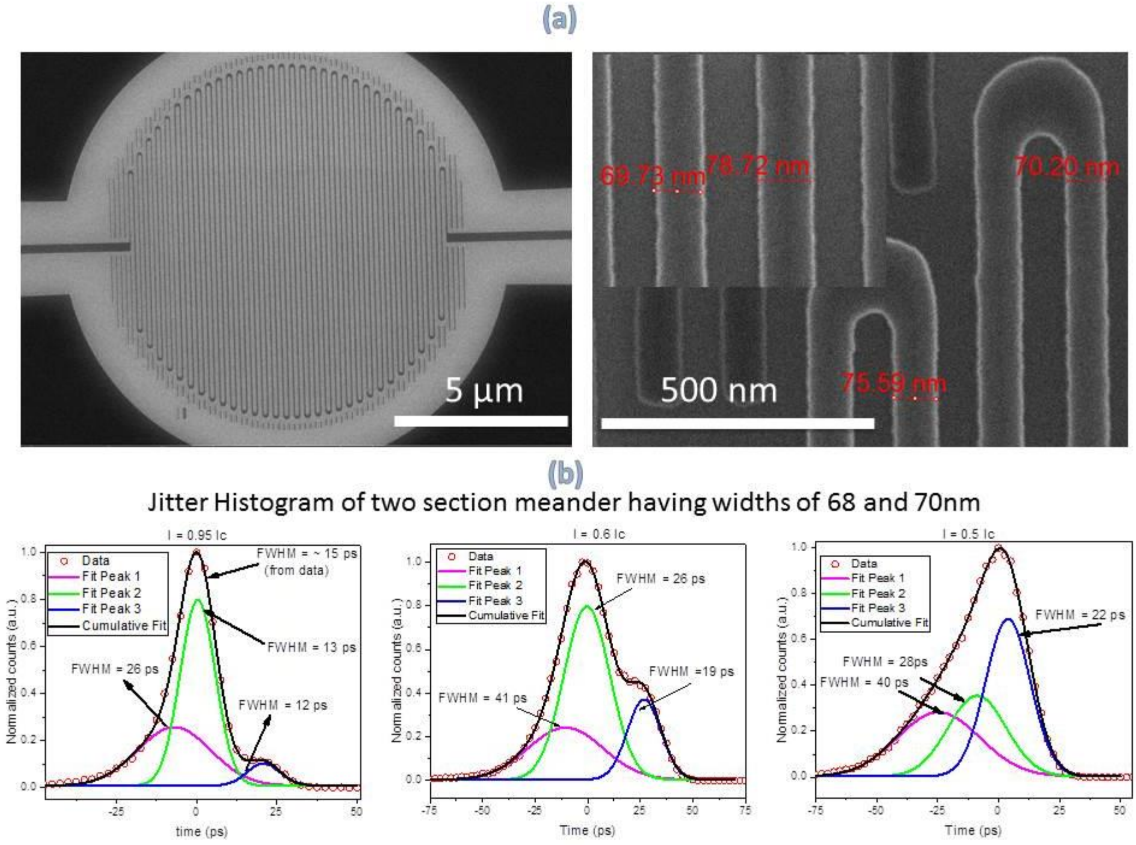


**Fig. S 7, (a) More (in addition to the ones shown in the main text) SEM images of a two sectioned detector. (b) time jitter versus bias current measurements for a two section SNSPD having widths difference of only 2nm (68nm wide and 70nm wide). The two peaks attributed to the two sections are clearly visible in the time jitter measurements even for such small width difference.**

## S2.5. The proximity effects

As discussed in the main text, the proximity effects can affect the linewidth of different parts of meandering nanowire. To simulate the proximity effects, we used Raith 150 e-beam lithography proximity correction software. The software provide a relative change to the ebeam dose to correct for undesired proximity effects. Fig. S 8 (a) show proximity effect corrections for a positive ebeam resist (CSAR, ARP series) with two different thicknesses and the same simulations for a negative ebeam resist (HSQ) is shown in Fig. S 8 (b) .

For ARP, the thinner resist is closer to the base dose (not much correction is required) but both cases have a good uniformity and therefore it is possible to optimize a single dose to get a

relatively uniform structure. In the case of HSQ, both thicknesses require higher doses than the base dose, however, the thinner resist presents better dose uniformity than the thicker resist (it is possible to get a relatively uniform writing by increasing the dose without correction).
Note that the non-symmetric shape of the dose distribution is due to the contour that e-beam follows to expose the structure. This contour creates a non-symmetric pattern of dose distribution as well as a non-symmetric heat profile during exposure. When correctly configured, the software is capable of correcting both dose and heat distributions.

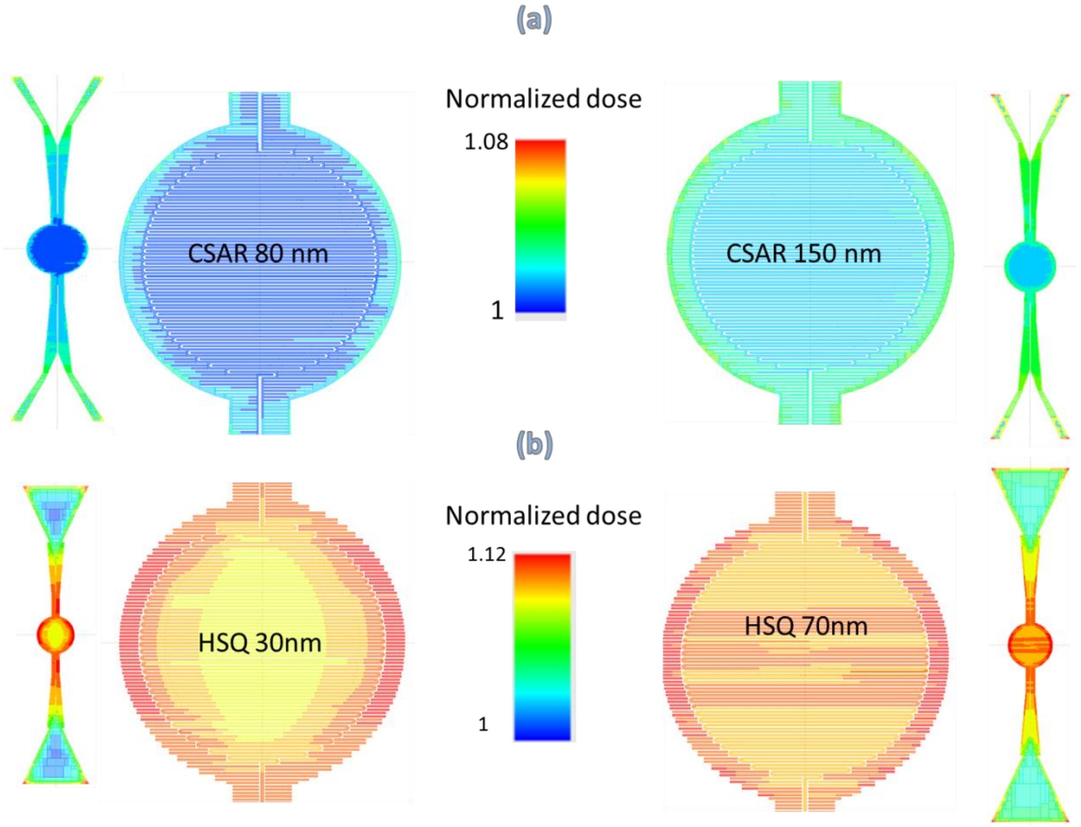


Fig. S 8, (a) Proximity effect correction for a positive ebeam resist (CSAR, ARP series) with two different thicknesses. The thinner resist is closer to the base dose (not much correction is required) but both have a good uniformity. (b) same as simulations for a negative ebeam resist (HSQ). Both thicknesses require higher doses that the base dose, however, the thinner resist presents better dose uniformity than the thicker resist (it is possible to get a relatively uniform writing by increasing the dose).

## S2.6. Simulation of jitter for two sectioned SNSPDs

As discussed in the main text, we simulated a two sectioned SNSPD by considering electronic-noise-induced timing jitter [3, 4], geometric timing jitter [5], and inhomogeneity-induced timing jitter [6]. Below is a list and the definition of parameters that are used in the simulations.

Table 1, A summary of parameters used in simulations.

| Symbol | Meaning |
|---|---|
| $d$ | Thickness of nanowire |
| $w$ | Width of nanowire |
| $j_{c0}$ | Critical current density at 0 K |
| $\rho_{10\,\mathrm{K}}$ | Resistivity at 10 K<br>(Not sheet resistance) |
| $L_{\mathrm{k}}$ | Kinetic inductance |
| α | Thermal boundary conductivity at 10 K |
| $c_{\mathrm{N}}$ | Normal state specific heat |
| $c_{\mathrm{S}}$ | Superconducting state specific heat |

| | |
|---|---|
| $\kappa_{\mathrm{N}}$ | Normal state thermal conductivity |
| $\kappa_{\mathrm{S}}$ | Superconducting state thermal conductivity |
| $T_{\mathrm{sub}}$ | Working temperature |
| $T_{\mathrm{c}}$ | Critical temperature |
| $C_{\mathrm{bt}}$ | Capacitance of bias tee |
| $I_{\mathrm{SW}}$ | Switching current |
| $j_{\mathrm{c}}$ | Critical current density |
| $V$ | Voltage |
| $\sigma_{\mathrm{N}}$ | Standard deviation of electric noise |
| $\mathrm{TJ}_{\mathrm{noise}}$ | Noise-induced timing jitter in standard deviation |
| $C_{\mathrm{g}}$ | Capacitance between nanowire and ground |
| $L_{\mathrm{g}}$ | Inductance of nanowire |
| $v$ | RF signal velocity along the nanowire |
| $\Delta t$ | Transmission-line-effect-induced time delay |
| $\mathrm{TJ}_{\mathrm{geometric}}$ | Transmission-line-effect-induced timing jitter in standard deviation |
| $\Delta$ | Superconducting gap |
| $\overline{w}$ | Mean of the distributed width |
| $\overline{d}$ | Mean of the distributed thickness |
| $\overline{\Delta}$ | Mean of the distributed superconducting gap |
| $\sigma_{w}$ | Standard deviation of the distributed width |
| $\sigma_{d}$ | Standard deviation of the distributed thickness |
| $\sigma_{\Delta}$ | Standard deviation of the distributed superconducting gap |
| $l_{\mathrm{g}}^{w}$ | Granularity[1] of the distributed width |
| $l_{\mathrm{g}}^{d}$ | Granularity[1] of the distributed thickness |
| $l_{\mathrm{g}}^{\Delta}$ | Granularity[1] of the distributed superconducting gap |
| $a$ | Gaussian fit parameter, no physical meaning |
| $t$ | Time |
| $t_1$ | Electro-thermal-evolution-induced time delay |
| $\mathrm{TJ}_{\mathrm{inhomogeneity}}$ | Inhomogeneity-induced timing jitter in standard deviation |
| $t_0$ | Overall time delay |
| $\mathrm{TJ}_{\mathrm{overall}}$ | Overall timing jitter in standard deviation |
| $F$ | Gaussian function |
| $A_0$ | Gaussian fit parameter, no physical meaning |
| DE | Detection efficiency |

1. The granularity is the characteristic length below which a property of the nanowire can be considered as being uniform and above which the property varies.

The total time jitter distribution can be constructed by considering all of above mentioned jitter contributions weighted by absorption and internal efficiencies of 70nm and 77nm wide sections:

### S2.6.1. Electro-thermal and geometric parameters

We followed [8] to simulate electrothermal evolution of the hotspot. For the critical current density, sheet resistance, kinetic inductance, we could get the numbers directly, for other electrothermal parameters, we used the values reported in [8] as initial guess and adjusted them to get better fit to the experimental pulses.

Geometric parameters

| $\bar{d}$ (nm) | $\bar{w}_1$ (nm) | $\bar{w}_2$ (nm) | $\mathrm{Length}_1$ (μm) | $\mathrm{Length}_2$ (μm) | $\mathrm{Area}_1$ (μm$^2$) | $\mathrm{Area}_2$ (μm$^2$) |
|---|---|---|---|---|---|---|
| 8.5 | 70 | 77 | 60.7 | 465 | 4.25 | 35.86 |

d = film thickness of the tested sample. $w_1$ & $w_2$ denote the nanowire width in the two section.

Area 1 = area covered by the narrower section (w1 = 70 nm)
Area 2 = area covered by the wider section (w2 = 77 nm)

## Electrothermal parameters

| $j_{c0}$ (nA/nm$^2$) | $\rho_{10\ K}$ (μΩ·cm) | $L_k$ (nH) | $\alpha$ (W/m$^2$K) | $c_N$ | $c_S$ | $\kappa_N$ | $\kappa_S$ | $T_{sub}$ (K) | $T_c$ (K) | $C_{bt}$ (nF) |
|---|---|---|---|---|---|---|---|---|---|---|
| 85 | 427 | 448 | $5.5\times10^5$ | $2c_N^*$ | $\frac{c_S^*}{4}$ | $\frac{\kappa_N^*}{2}$ | $2\kappa_S^*$ | 2.8 | 10.5 | 20 |

* in the table denotes the values reported in [8]. Here $j_{c0}$ denotes the critical current density at zero temperature (T= 0 K). $\rho_{10\ K}$ is the sheet resistance at T = 10K. $c_N$, $c_S$, $k_N$, $k_S$ represent thermal boundary conductivity, specific heat in superconducting state, specific heat in normal state, normal state thermal conductivity, and superconducting state thermal conductivity, respectively.

The measured switching current was $I_{sw} = 38.9\ \mu A$ at $T = 2.8\ K$, which was limited by the 70-nm part of the hybrid SNSPD. Therefore, the switching current density at $T = 2.8\ K$ was $j_c = \frac{I_{sw}}{w_{min} d_{min}} = 73.4\ nA/nm^2$. The switching current density at $T = 0$, $j_{c0}$ was calculated by: $j_{c0} = \frac{j_c}{\left(1-\left(\frac{T}{T_c}\right)^2\right)^2}$,

and $j_c$ at other temperature was calculated using: $j_c = j_{c0} \cdot \left(1-\left(\frac{T}{T_c}\right)^2\right)^2$.

Our adjustment of parameters includes: a=5.5E5 W/m$^2$K, $c_N$=2$c_N$*, $c_S$=$c_S$*/4, $k_N$=$k_N$*/2, $k_S$=2$k_S$*.

The slew rate of the simulated pulse at (6.5 V/ns) was close to that of experimental pulse (6.76 V/ns), Fig. S 9, and this was achieved by considering the Gain of the amplifier to be 64.5 dB (slightly higher than measured ~62dB). The Gain spectrum of the amplifier was not considered in this simulation.

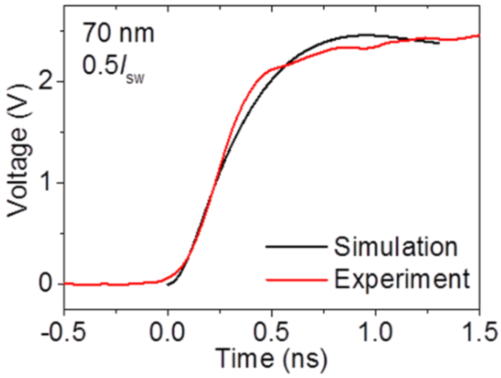


**Fig. S 9, The fit to a detection pulse of the detector was used to adjust eletrothermal simulation parameters.**

We used the noise level at the output of the amplifier, as shown in Fig. S 10, and calculated back the input referred noise (dividing by gain of the amplifier). The input noise level was used to calculate the electronic noise induced jitter,

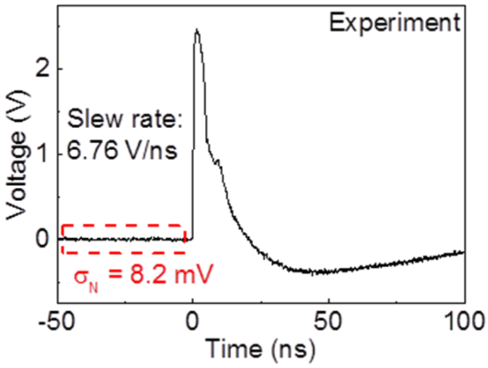


**Fig. S 10, We calculated input referred noise from the output pulse noise level ($\sigma_N$) and the gain of the amplifier.**

The electronic noise induced jitter was then simulated by considering a Gaussian distribution function for voltage noise:

Noise is Gaussian function: $e^{-\frac{(V-\bar{V})^2}{2\sigma_N^2}}$

The slew rate depends on the bias and the nanowire width. Therefore for each section of the nanowire and for each bias current we can calculate an “effective time delay”: $\mathrm{TJ_{noise}} = \frac{\sigma_\mathrm{N}}{\mathrm{Slew\ rate}}$

The results are shown in Fig. S 11.

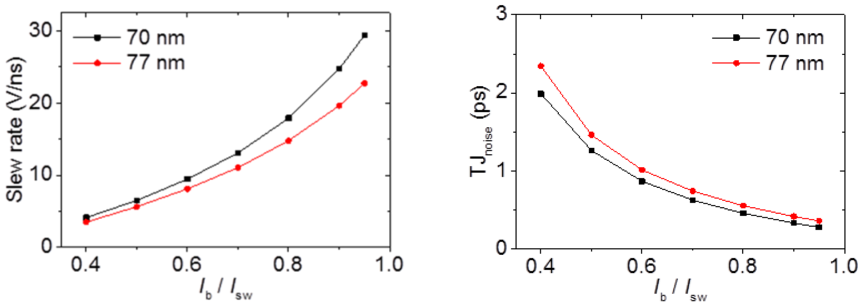


**Fig. S 11, Simulated slew rate and time delay for the two sections of the nanowire.**

The deviation of these values from experimental observation could have been caused by an imperfect fit to the experimental pulses.

### S2.6.2. The transmission line effect

The detection events taking place in different parts of the nanowire would experience a different transmission line length to the readout output. The amount of such delay depends on the kinetic inductance of nanowire sections and the capacitance between nanowire sections and the ground. For consistency, here we follow literature in calculating the transmission line effect (despite our experimental observation about the low timing jitter suggesting possible different mechanisms for the propagation of detection pulses). Fig. S 12 shows our model to calculate the transmission line delay. Note that, since the thickness of Si is ~1000 times larger than the thickness of $SiO_2$ (which is between the NbTiN layer and Silicon in real devices), $SiO_2$ was excluded from the capacitance calculation.

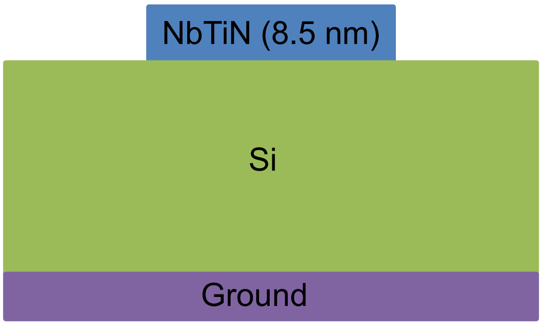


**Fig. S 12, Our model for calculating transmission line effect.**

Using AppCAD™ to calculate the capacitance per length, we get: $C_{g\ 70}$: 35.32 pF/m, and $C_{g\ 77}$: 35.65 pF/m and Kinetic inductance per length was calculated from the pulse decay to be: $L_{g\ 70}$: 0.93 nH/□m , $L_{g\ 77}$: 0.84 nH/□m. This gives:

RF signal velocity: $v = \frac{1}{\sqrt{C_g \cdot L_g}}$ → $v_{70}$: 1.84% $c$ , $v_{77}$: 1.92% $c$

flood illumination →

The time delay along the nanowire is a uniform distribution:

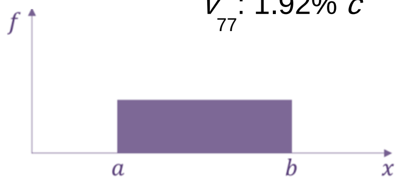


Probability density function: $f = \frac{1}{b-a}$ Mean: $E(x) = \int_a^b x \cdot f(x)\,\mathrm{d}x = \frac{1}{b-a}\int_a^b x\,\mathrm{d}x = \frac{a+b}{2}$

Standard deviation: $Std = \sqrt{\int_a^b [x - E(x)]^2 \cdot f(x)\,\mathrm{d}x} = \sqrt{\frac{1}{b-a}\int_a^b \left(x - \frac{a+b}{2}\right)^2 \mathrm{d}x} = \frac{b-a}{2\sqrt{3}}$

However, this does not match our experimental observation Fig. S 14. A Gaussian distribution match our experimental results better.

### S2.6.3. The effect of inhomogeneity

The probability density of $w$, $d$ and $\Delta$ along the nanowire are considerd to be Gaussian functions: $e^{-\frac{(w-\bar{w})^2}{2\sigma_w^2}}$, $e^{-\frac{(d-\bar{d})^2}{2\sigma_d^2}}$, and $e^{-\frac{(\Delta-\bar{\Delta})^2}{2\sigma_\Delta^2}}$.

| $\sigma_w/\bar{w}$ | $\sigma_d/\bar{d}$ | $\sigma_\Delta/\bar{\Delta}$ | $l_g^w$ (nm) | $l_g^d$ (nm) | $l_g^\Delta$ (nm) |
|---|---|---|---|---|---|
| 1% | 2% | 5% | 5 | 5 | 50 |

We use the function $f = a \cdot \exp[-\frac{1}{2}\left(\frac{t-t_1}{\mathrm{TJ}_{inhomogeneity}}\right)^2]$ to fit the histograms from electro-thermal simulation, the fitting parameters are listed in the following table: (the inflection at 0.3$I_{sw}$ is due to the use of Gaussian functions to fit the simulated histogram with exponential tail)

| $I_b$ / $I_{sw}$ | 70 nm | | | 77 nm | | |
|---|---|---|---|---|---|---|
| | $a$ | $t_1$ | $\mathrm{TJ}_{inhomogeneity}$ | $a$ | $t_1$ | $\mathrm{TJ}_{inhomogeneity}$ |
| 0.4 | 0.1101 | 325.4 | 8.39336 | 0.1157 | 365.7 | 9.56715 |
| 0.5 | 0.08501 | 274.4 | 7.55897 | 0.09649 | 309.9 | 8.18123 |
| 0.6 | 0.0833 | 237.3 | 6.1391 | 0.07957 | 270.5 | 7.2832 |
| 0.7 | 0.0898 | 205.7 | 4.67256 | 0.08936 | 238.5 | 5.66958 |
| 0.8 | 0.08312 | 176.4 | 3.70524 | 0.08543 | 209.5 | 4.4873 |
| 0.9 | 0.09 | 147.7 | 3.06248 | 0.08506 | 182 | 3.70948 |
| 0.95 | 0.09381 | 132.9 | 2.65377 | 0.08978 | 168.3 | 3.38633 |

### S2.6.4. The effect of internal efficiency

The contribution of each of 70nm and 77nm wide sections to the overall jitter is determined by both the active area of each section and its relative internal efficiency.

The relative total detection efficiency determines the area under curve for each peak in the overall jitter histogram. Therefore, a good estimation for the internal efficiency of each section is required to match the experimental data. Fig. S 13 shows internal efficiency (measured and fitted) for a test sample and the relative total efficiency curves (calculated by also taking into account the absorption for different sections) used in our simulations .

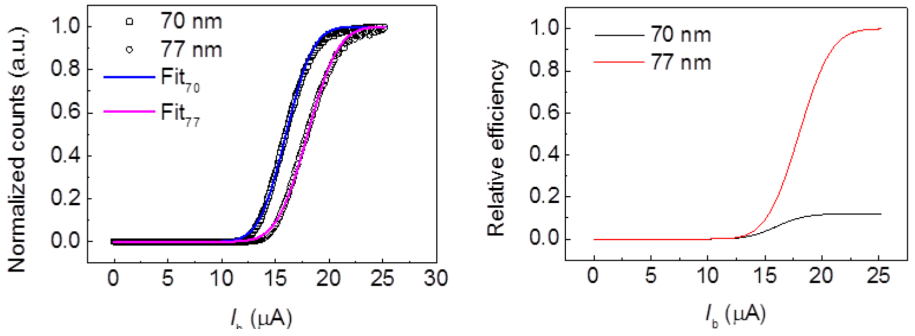


**Fig. S 13, Internal efficiency (measured and fitted) and relative total efficiency curves (calculated by taking into account the absorption for different sections) for a test sample.**

### S2.6.5. The overall jitter

The overall time delay is calculated from the rising edge of the signal (electro-thermal evolution) and the transmission line effect:

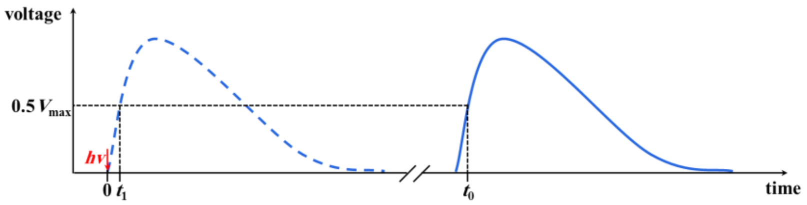


$0 \rightarrow t_1$: electro-thermal evolution

$t_1 \rightarrow t_0$: transmission line effect, D*t*

$0 \rightarrow t_0$: overall time delay

$$t_0 = t_1 + \Delta t$$

Similarly the overall time jitter can be calculated as following:

$$\mathrm{TJ}_{\text{overall}} = \sqrt{\mathrm{TJ}_{\text{noise}}^2 + \mathrm{TJ}_{\text{geometric}}^2 + \mathrm{TJ}_{\text{inhomogeneity}}^2}$$

For each bias current, we can get two functions for 70nm wide and 77nm wide sections, Each function has such form:

$$F = A_0 \cdot \exp[-\frac{1}{2}\left(\frac{t - t_0}{\mathrm{TJ}_{\text{overall}}}\right)^2]$$

$A_0$ is determined by the relative efficiency between 70 and 77: $\frac{\int F_{70}\,\mathrm{d}x}{\int F_{77}\,\mathrm{d}x} = \frac{DE_{70}}{DE_{77}}$ .

the overall histograms are given by: $F_{70} + F_{77}$. Finally, by considering all contributions we end up in the final simulation results as shown in the Fig. S 14. One can observe that the results by excluding transmission line effect is closer to our experimental observations (see the main text).

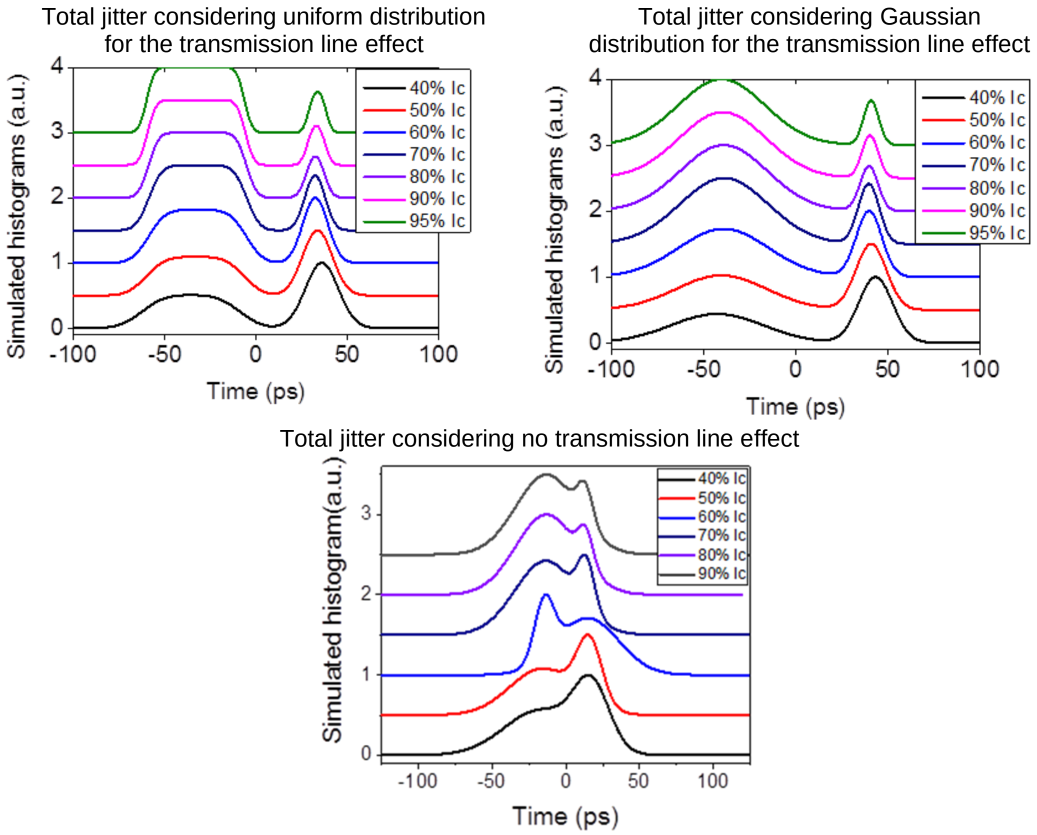


**Fig. S 14, Total jitter considering uniform and Gaussian distribution for the transmission line effect. The latter provides a better agreement with our experimental observations. The closest match can be made when not including the transmission line effect at all.**

# S3- Multi-pixel SNSPDs

## S3.1. RF crosstalk and device performance at different wavelength

RF crosstalk between the pixels is a major concern. If the signal routings are next to one another with no grounding in between, a significant crosstalk is observed, as shown in Fig. S 15(a), while adding the ground lines in between (at least ~3x thicker than nanowire width) ensures a crosstalk-free performance, Fig. S 15(b).

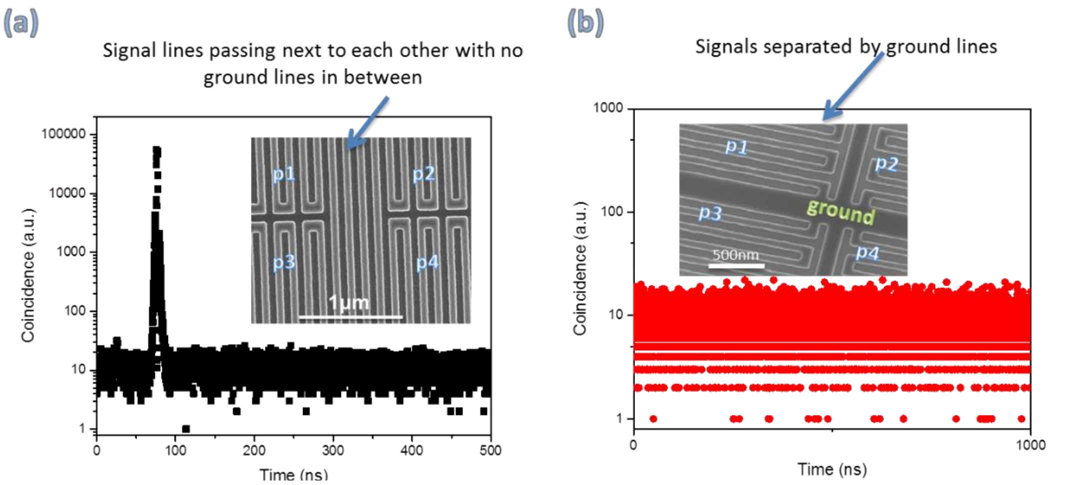


Fig. S 15, Cross talk measurement for two devices: (a) without grounding between signal lines, exhibiting a high level of crosstalk, and (b) with grounding between pixels with no noticeable crosstalk.

## S3.2. 16-pixel SNSPD performance at different wavelength

We measured our 16-pixel device at other wavelength that is mentioned in the main text (660nm). The performance is similar, however, due to the multimode illumination (an SMF28 fiber placed far from the sample was used to illuminate the sample), some pixels get slightly higher photon flux than the other ones depending on the wavelength and the excited modes at the launch.

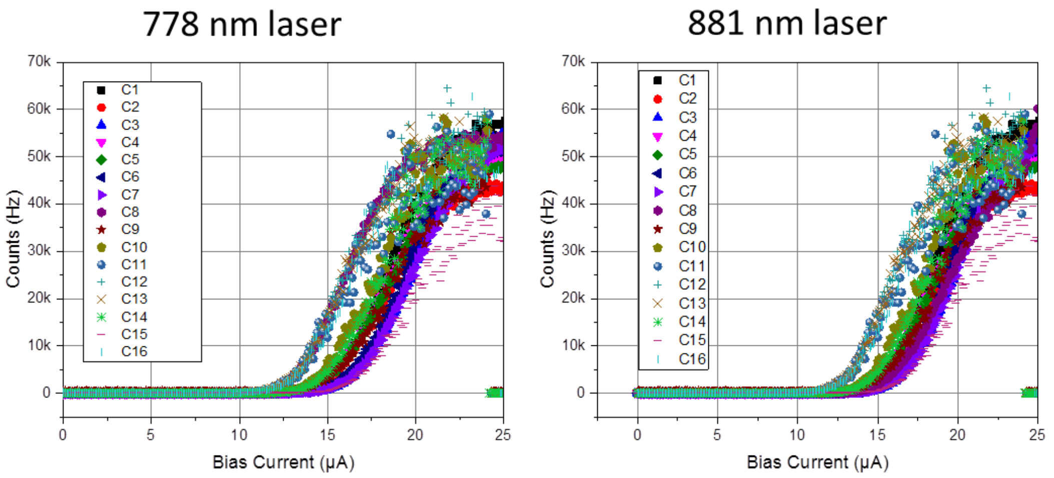


Fig. S 16, photon count rate measurement for the 16-pixel device at two wavelengths of 778nm and [illegible]

## S3.3. Photon antibunching with multi-pixel detectors

As discussed in the main text, we performed antibunching measurement on a nanowire quantum dot. The emission spectrum of the quantum dot and the unprocessed antibunching data (for the same pairs of detectors as discussed in the main text) are shown in Fig. S 17 (a) and (b) respectively.

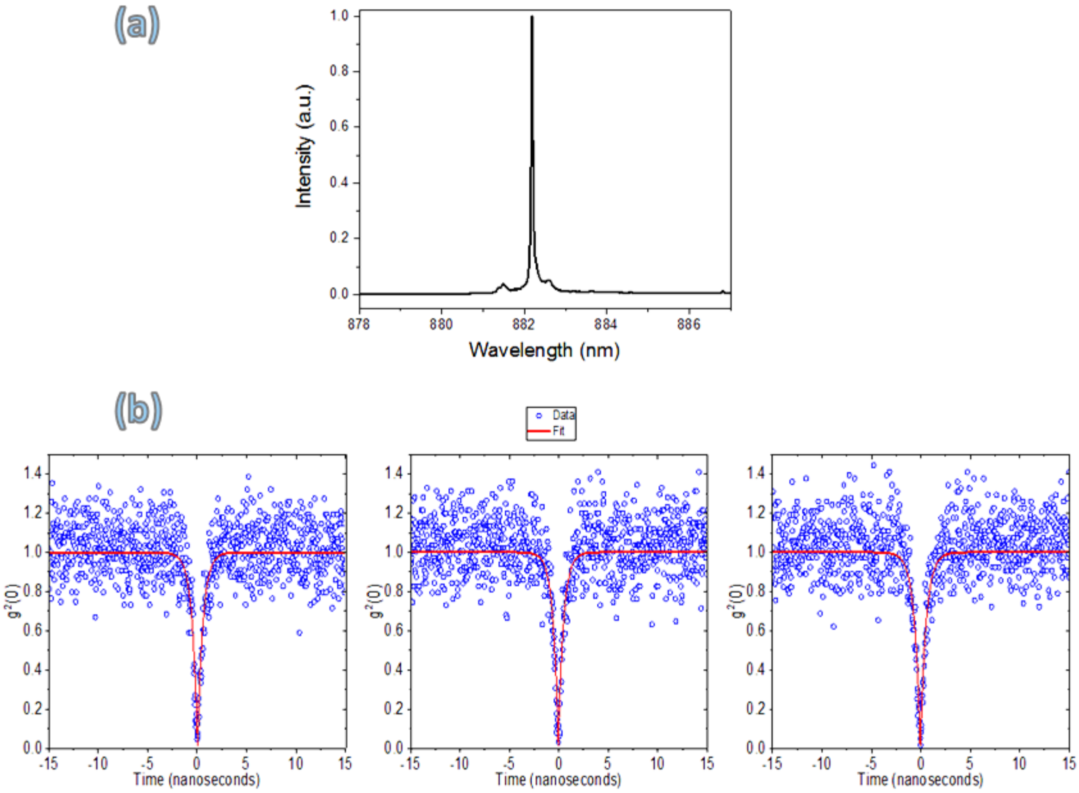


**Fig. S 17, (a) Emission spectrum of nanowire quantum dot used in the antibunching experiment. (b) unprocessed data of correlation measurements for the same pairs as the main text.**

It was mentioned in the main text that the overall time jitter of the experiment was limited by the time dispersion of spectrometer. We used an 1800 grooves per mm grating, kept the input slit of the spectrometer fixed at 50μm and varied the size of output slit. Below are our experimental observations for different output slit sizes:

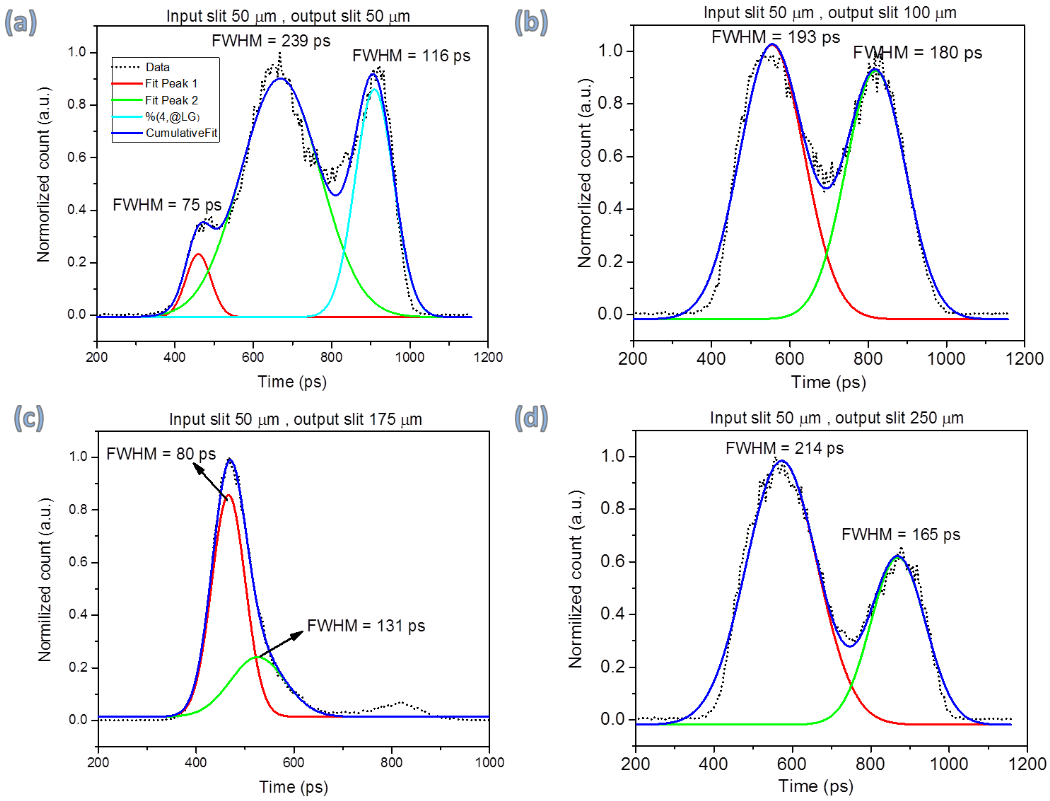


**Fig. S 18, spectrometer time dispersion a function of monochromator output slit size.**

The direct time jitter measurement on the detector yielded ~60ps time resolution (no cryoamp was used) both using a single mode and multimode fiber coupling.

## Bibliography


[1] I. E. Zadeh, J. W. N. Los, R. B. M. Gourgues, V. Steinmetz, G. Bulgarini, S. M. Dobrovolskiy, V. Zwiller and S. N. Dorenbos, "Single-photon detectors combining high efficiency, high detection rates, and ultra-high timing resolution," *APL Photonics,* vol. 2, no. 11, 2017.

[2] M. Sidorova, A. Semenov, H.-W. Hübers, I. Charaev, A. Kuzmin, S. Doerner and M. Siegel, "Physical mechanisms of timing jitter in photon detection by current-carrying superconducting nanowires," *Phys. Rev. B,* vol. 96, no. 18, 2017.

[3] Q. Zhao, L. Zhang, T. Jia, L. Kang, W. Xu, J. Chen and P. Wu, "Intrinsic timing jitter of superconducting nanowire single-photon detectors," *Applied Physics B,* vol. 104, no. 3, pp. 673-678, 2011.

[4] L. You, X. Yang, Y. He, W. Zhang, D. Liu, W. Zhang, L. Zhang, L. Zhang, X. Liu, S. Chen, Z. Wang and X. Xie, "Jitter analysis of a superconducting nanowire single photon detector," *AIP Advances,* vol. 3, no. 7, p. 072135, 2013.

[5] N. Calandri, Q.-Y. Zhao, D. Zhu, A. Dane and K. K. Berggren, "Superconducting nanowire detector jitter limited by detector geometry," *Applied Physics Letters,* vol. 109, no. 15, p. 152601, 2016.

[6] Y. Cheng, C. Gu and X. Hu, "Inhomogeneity-induced timing jitter of superconducting nanowire single-photon detectors," *Applied Physics Letters,* vol. 111, no. 6, p. 062604, 2017.

[7] J. K. W. Yang, A. J. Kerman, E. A. Dauler, V. Anant, K. M. Rosfjord and K. K. Berggren, "Modeling the Electrical and Thermal Response of Superconducting Nanowire Single-Photon Detectors," *IEEE Transactions on Applied Superconductivity,* vol. 17, no. 2, pp. 581-585, 2007.

[8] J. Chang, I. E. Zadeh, J. W. N. Los, J. Zichi, A. Fognini, M. Gevers, S. Dorenbos, S. F. Pereira, P. Urbach and V. Zwiller, "Multimode-fiber-coupled superconducting nanowire single-photon detectors with high detection efficiency and time resolution," *Applied Optics,* vol. 58, no. 36, pp. 9803-9807, 2019.
